# Supplementary material for: Spontaneous Demixing of Binary Colloidal Flocks
Source: arXiv:2306.15614 source file (2023-11-24)
Supplement: Supplementary file 1 [file Maity2023_Supplementary_Information.pdf]

# Supplemental Materials

## Spontaneous Demixing of Binary Colloidal Flocks

Samadarshi Maity and Alexandre Morin\*  
*Huygens-Kamerlingh Onnes Laboratory, Universiteit Leiden,*  
*PO Box 9504, 2300 RA Leiden, the Netherlands*  
(Dated: November 24, 2023)

### CONTENTS

|                                                                    |    |
|--------------------------------------------------------------------|----|
| A. Experiments                                                     | 2  |
| 1. Methods and materials                                           | 2  |
| a. Materials                                                       | 2  |
| b. Microfluidic device                                             | 2  |
| c. Analysis techniques                                             | 3  |
| d. Self propulsion speed and rotational diffusivity                | 3  |
| 2. Transient dynamics                                              | 3  |
| 3. Flocking transition                                             | 4  |
| 4. Robustness of demixing to particle material and mixture ratio   | 4  |
| B. Theory: Microscopic dynamics of mixtures                        | 5  |
| 1. Generalities: from individual dynamics to pairwise interactions | 5  |
| a. Quincke electro-rotation                                        | 5  |
| b. Individual dynamics                                             | 6  |
| c. Pairwise interactions                                           | 6  |
| 2. Hydrodynamic alignment interactions                             | 7  |
| a. Response                                                        | 7  |
| b. Perturbation                                                    | 7  |
| c. Pairwise alignment                                              | 7  |
| 3. Electrical repulsive interactions                               | 7  |
| a. Response                                                        | 7  |
| b. Perturbation                                                    | 8  |
| c. Pairwise repulsion                                              | 8  |
| 4. Equations of motions                                            | 8  |
| C. Theory: Hydrodynamics of binary mixtures                        | 9  |
| 1. Coarse-graining the microscopic dynamics                        | 9  |
| 2. Evolution equation for the polarization                         | 9  |
| 3. Hydrodynamic equations in polar geometry                        | 11 |
| 4. Hydrodynamics of colloidal flocks                               | 11 |
| 5. Non-reciprocity driven demixing                                 | 14 |
| D. Experiments: Measurements of the hydrodynamic coefficients      | 15 |
| 1. Alignment interactions                                          | 15 |
| 2. Repulsive interactions                                          | 16 |
| E. Description of the Supplementary Movie                          | 18 |
| References                                                         | 18 |

## Appendix A: Experiments

### 1. Methods and materials

#### a. Materials

Binary polar fluids are assembled from polystyrene colloids of two different diameters:  $6.9 \pm 0.5 \mu\text{m}$  (Thermo Scientific 2005ATS) and  $10.1 \pm 5\% \mu\text{m}$  (Thermo Scientific G1000). The  $10 \mu\text{m}$  particles are fluorescent whereas the  $7 \mu\text{m}$  particles are non-fluorescent for efficient identification and tracking. The colloidal mixture is suspended in a weakly conducting non-polar medium consisting of  $0.14 \text{ mol l}^{-1}$  of sodium dioctyl sulfosuccinate (Sigma Aldrich) and  $0.03 \%$  (v/v) of de-ionized water dissolved in pure hexadecane (Sigma Aldrich).

We further check the monodispersity of the two species by optical microscopy and scanning electron microscopy in Fig. 1. The analysis of the colloidal particle sizes based on the optical images confirms the narrow distributions reported by the manufacturer. A slight shift towards larger values is an optical effect. Scanning electron microscopy images indeed confirms the mean values reported by the manufacturer.

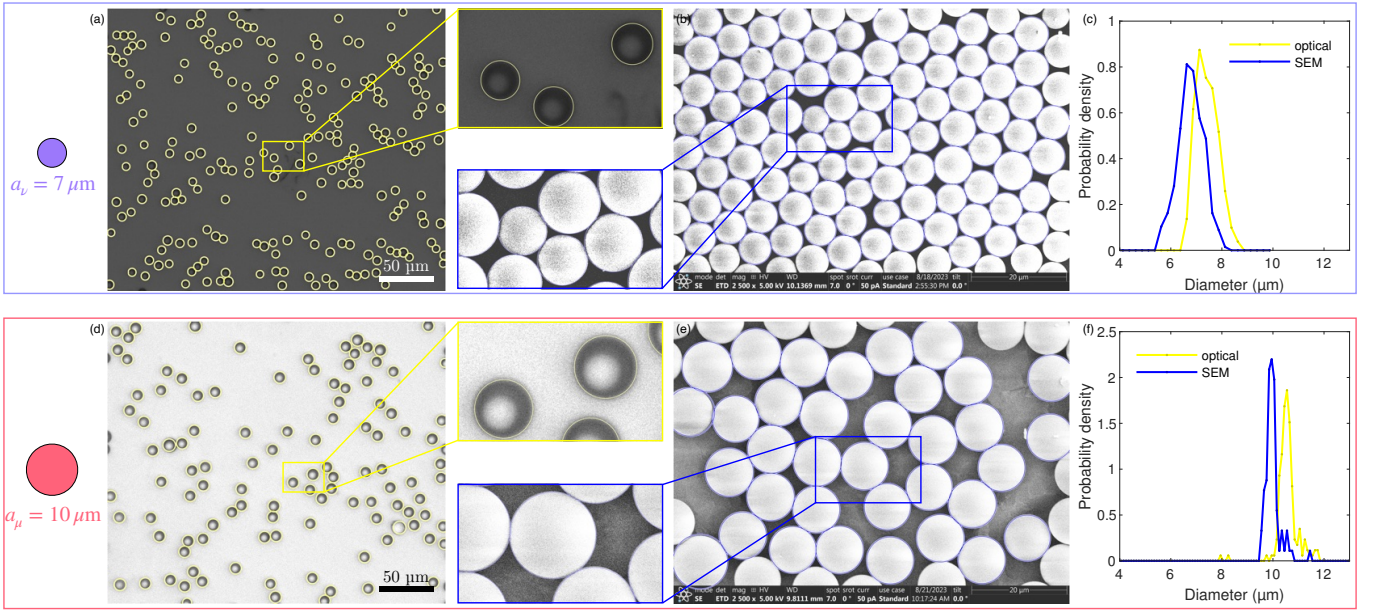

FIG. 1. Size of the colloidal particles. Top row:  $7 \mu\text{m}$ -diameter particles. Bottom row:  $10 \mu\text{m}$ -diameter particles. (a) Optical micrograph. (b) Scanning electron micrograph. (c) Size distributions obtained by optical microscopy (yellow,  $7.4 \pm 0.4 \mu\text{m}$ , obtained over 526 particles) and scanning electron microscopy (blue,  $6.8 \pm 0.5 \mu\text{m}$ , obtained over 271 particles). (d-f) Same as top row for the  $10 \mu\text{m}$ -diameter particles (yellow:  $10.6 \pm 0.4 \mu\text{m}$  obtained over 172 particles; blue:  $10.0 \pm 0.3 \mu\text{m}$ , obtained over 91 particles).

#### b. Microfluidic device

Microfluidic devices are fabricated using two horizontally parallel glass slides coated with a thin, conducting layer of indium tin oxide and (ITO) (Solems, ITOSOL30, ITO layer thickness:  $80 \text{ nm}$ ). These two electrodes are assembled using a double-sided, adhesive tape with a uniform thickness of  $50 \mu\text{m}$ . The bottom electrode is patterned with circular wells of diameter  $d$  ranging from  $2.1 \text{ mm}$  to  $8.4 \text{ mm}$ . The wells are constructed using a positive photoresist resin (Microposit S1818, thickness:  $4.5 \mu\text{m}$ ) through the conventional ultraviolet lithography technique. Binary mixtures of colloidal particles are injected into the microfluidic device and the colloids eventually deposit into the circular wells. Polystyrene colloidal particles are turned into self-propelled particles by mean of the Quincke electro-rotation instability, see Section B. They are powered by application of a uniform D.C. electric field  $\mathbf{E}$  transverse to the two electrodes using a voltage amplifier (B.K. Precision, 9185B). All reported measurements correspond to an applied electric field of  $|\mathbf{E}| = 3.4 \pm 5\% \text{ V}/\mu\text{m}$ . The dynamics of the colloidal rollers is observed using magnifications between 2X to 6X and recorded using a CMOS camera (XIMEA xiX) fitted to a stereo microscope (NIKON SMZ18)

with frame rates ranging between 200 to 450 Hz. For the largest confinement i.e.  $d = 8.4$  mm, the processing data are stitched together from different image sequences recorded from different sections of this circular confinement due to limitations in the size of the observation window. The observation window spans  $1024 \text{ pixels} \times 2464 \text{ pixels}$  where 1 pixel corresponds to  $0.862 \mu\text{m}$  for 2X magnification.

### c. Analysis techniques

The analysis and measurement of parameters are undertaken on the image sequences recorded after the system has reached its steady state, see Fig. 2. The particle coordinates are identified on each frame using ImageJ. Trajectories are subsequently reconstructed using Python and Matlab routines implementing the traditional Crocker and Grier algorithm [1]. Finally, all subsequent calculations are performed using Python or MATLAB conveniently using their standard toolkits for statistical computations.

### d. Self propulsion speed and rotational diffusivity

The self-propulsion speed of the particles is measured from their displacements over 6 ms- to 13 ms-long time intervals, depending on the recording frame rate, which is much shorter than their persistence length. Values reported in the main text are time and ensemble averages.

The rotational diffusivity  $D$  of the binary mixture is measured under extremely dilute conditions (total density  $\rho_{\mu+\nu} \sim 10^{-5} \mu\text{m}^{-2}$ ) to minimize the contributions to the rotational noise due to inter-particle collisions.  $D$  is obtained by measuring the ensemble average of the auto-correlation of the particle orientations  $\hat{\mathbf{v}}_i$ , such that:

$$\langle \hat{\mathbf{v}}_i(t_0) \cdot \hat{\mathbf{v}}_i(t_0 + t) \rangle_{i,t_0} = \exp(-Dt). \quad (\text{A1})$$

The direction of motion of the  $10 \mu\text{m}$  particles freely diffuses on the unit circle with  $D = 1.9 \pm 15\% \text{ s}^{-1}$  whereas, for  $7 \mu\text{m}$  particles,  $D = 3.4 \pm 15\% \text{ s}^{-1}$ .

## 2. Transient dynamics

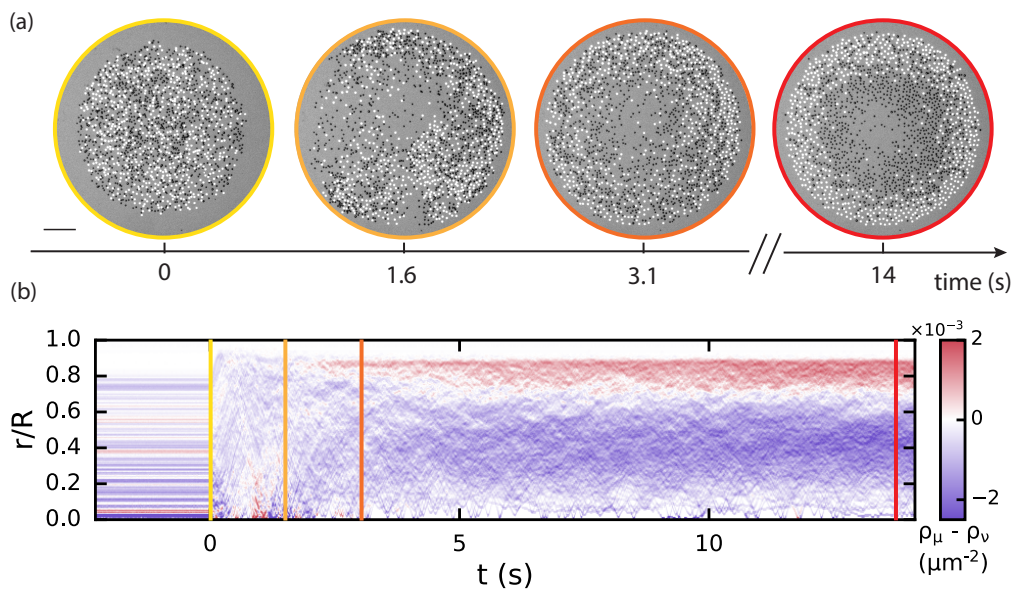

FIG. 2. Transient evolution of a binary colloidal flock confined in a circular well of radius  $R = 0.6$  mm. (a) Experimental snapshots (main text Fig. 1(a)). Scale bar:  $200 \mu\text{m}$ . (b) Time evolution of the radial profile of the density difference  $\rho_{\mu} - \rho_{\nu}$ . The vertical lines indicate the times of the snapshots. The binary mixture quickly flocks, and subsequently self-sorts.

Upon application of DC electric field  $E = 3.4 \text{ V}/\mu\text{m}$ , higher than the Quincke threshold ( $E_{Q,10\mu\text{m}} = 2.15 \text{ V}/\mu\text{m}$  and  $E_{Q,7\mu\text{m}} = 1.95 \text{ V}/\mu\text{m}$ ) of each species, particles start rolling on the substrate in all directions. Quickly, patches of coordinated motion appear, as seen on Fig. 2 at  $t = 1.6 \text{ s}$ . Hydrodynamic interactions favoring the alignment of the particle directions of motion promote the flocking: within the circular well, colloidal rollers form a vortex, see Fig. 2 at  $t = 3.1 \text{ s}$ . Within this vortex, the two species eventually demix, see Fig. 2 at  $t = 14 \text{ s}$ . As shown on the kymograph of Fig. 2, flocking precedes demixing.

### 3. Flocking transition

Binary mixtures of colloidal rollers undergo a flocking transition similar to the single species cases, as shown in Fig. 3 for 50:50 mixtures. At low density, the rollers form an homogeneous and disordered gas (panel (a)). At high density, they form a polar flock which takes the form of a vortex given the circular confinement (panel (c)). At intermediate density (panel (b)), the system spontaneously breaks rotational symmetry which is captured by the bifurcation of the polarization (panel (d)). At the transition, alignment interactions overcome rotational diffusion. The competition between the two dictates the evolution of the polarization, see Section C and in particular Eq. C24.

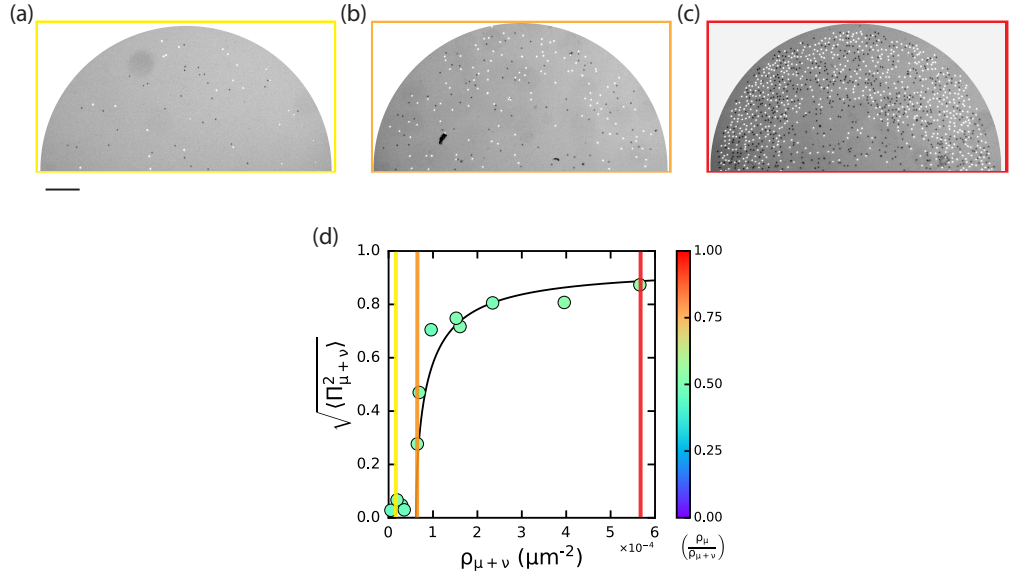

FIG. 3. Flocking transition of a 50:50 mixture confined in a circular well of radius  $R = 1.05 \text{ mm}$ . (a)-(c) Snapshots showing half the confinement wells for mixtures of increasing densities. Scale bar:  $250 \mu\text{m}$ . (a) Gas state. (b) Transition. (c) Polar vortex. (d) The polarisation of the 50:50 mixture bifurcates upon increasing the total density. The dots are colored according to the relative density, see colorbar. The vertical lines indicate the snapshots of panel (a), (b) and (c). The black solid line is the theoretical prediction  $\sqrt{\langle \Pi^2 \rangle} = (1 - 2D/(\rho_{\mu+\nu}(\alpha_{\mu\mu} + \alpha_{\nu\nu})))^{1/2}$  following from Eq. C24.

### 4. Robustness of demixing to particle material and mixture ratio

To test the robustness of the spontaneous demixing of binary polar liquids, we perform experiments with another set of colloidal particles. In place of the commercial polystyrene particles used in the Main text, we use home-made 3-(trimethoxysilyl)propyl meth-acrylate (TPM) colloids, synthesized following [2]. The resulting mixtures, of size  $6 \pm 0.8 \mu\text{m}$  and  $4.5 \pm 0.2 \mu\text{m}$  diameters, form colloidal flocks whose constituents spontaneously demix, see Fig. 4.

Figure 5 shows the radial density profiles of  $10 \mu\text{m}$ -diameter and  $7 \mu\text{m}$ -diameter polystyrene particles forming flocks of different mixing proportions. Demixing occurs for various mixing ratios and confinement sizes: the larger species tends to accumulate more towards the edge of the confinement than the other. The resulting radial density profiles depend on the precise density ratio.

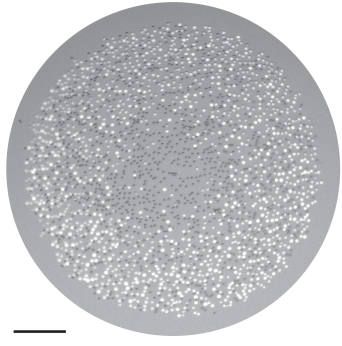

FIG. 4. TPM-colloid binary flock self-demixes. The larger, fluorescent, particles accumulate towards the edge. The smaller, non-fluorescent, particles accumulate in the core. Scale bar:  $200\ \mu\text{m}$ .

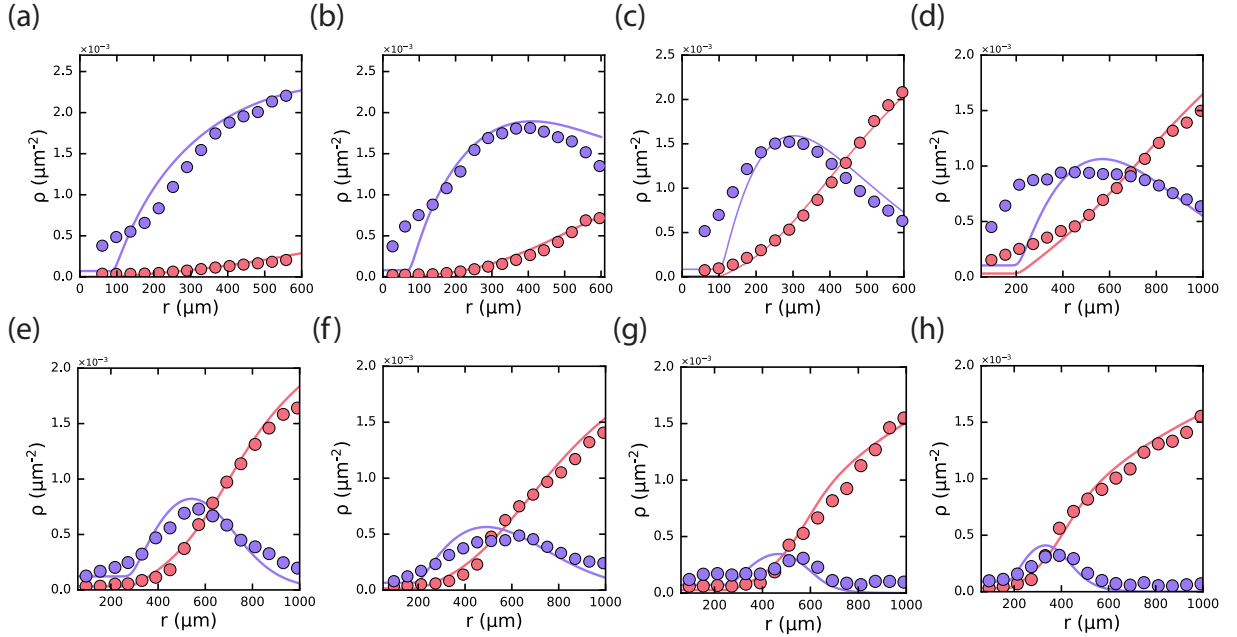

FIG. 5. Radial density profiles at steady-state for binary flocks of different mixtures. (a)  $N_\mu/N_{\mu+\nu} = 8.7\%$ ,  $v_\mu = 0.81\ \text{mm/s}$ , and  $v_\nu = 0.77\ \text{mm/s}$ . (b)  $N_\mu/N_{\mu+\nu} = 18\%$ ,  $v_\mu = 0.85\ \text{mm/s}$ , and  $v_\nu = 0.78\ \text{mm/s}$ . (c)  $N_\mu/N_{\mu+\nu} = 50\%$ ,  $v_\mu = 0.90\ \text{mm/s}$ , and  $v_\nu = 0.79\ \text{mm/s}$ . (d)  $N_\mu/N_{\mu+\nu} = 63\%$ ,  $v_\mu = 0.88\ \text{mm/s}$ , and  $v_\nu = 0.73\ \text{mm/s}$ . (e)  $N_\mu/N_{\mu+\nu} = 79\%$ ,  $v_\mu = 0.89\ \text{mm/s}$ , and  $v_\nu = 0.78\ \text{mm/s}$ . (f)  $N_\mu/N_{\mu+\nu} = 85\%$ ,  $v_\mu = 0.88\ \text{mm/s}$ , and  $v_\nu = 0.68\ \text{mm/s}$ . (g)  $N_\mu/N_{\mu+\nu} = 90\%$ ,  $v_\mu = 0.89\ \text{mm/s}$ , and  $v_\nu = 0.69\ \text{mm/s}$ . (h)  $N_\mu/N_{\mu+\nu} = 95\%$ ,  $v_\mu = 0.91\ \text{mm/s}$ , and  $v_\nu = 0.69\ \text{mm/s}$ . Confinement size:  $d = 1.2\ \text{mm}$  (a)-(c),  $d = 2.1\ \text{mm}$  (d)-(h). Violet:  $7\ \mu\text{m}$ -diameter colloidal particles. Red:  $10\ \mu\text{m}$ -diameter colloidal particles. Markers: experimental data. Lines: theory. See Fig. 9 for the corresponding particle fraction profiles.

## Appendix B: Theory: Microscopic dynamics of mixtures

### 1. Generalities: from individual dynamics to pairwise interactions

#### a. Quincke electro-rotation

The Quincke electro-rotation consists in the steady rotation at rate  $\Omega$  of a particle suspending in a fluid under the application of a DC electric field  $\mathbf{E}$ . This rotation results from an electro-hydrodynamic instability and spontaneously breaks the system rotational symmetry: the rotation takes place, randomly, around *any* axis perpendicular to the applied field ( $\boldsymbol{\Omega} \cdot \mathbf{E} = 0$ ). The essence of Quincke rotation can be highlighted by considering an electrically insulating

particle of dielectric permittivity  $\epsilon_s$  immersed in an unbounded fluid of permittivity  $\epsilon_s$  and electrical conductivity  $\sigma_1$ . Applying a DC electric field  $\mathbf{E}$  leads to the accumulation of charges at the fluid-particle interface. For an immobile particle, the resulting distribution is dipolar, and the dipole  $\mathbf{P}$  opposes the electric field:  $\mathbf{P} \cdot \mathbf{E} < 0$ . This situation forms the basis of the Quincke instability:

- Destabilization mechanism: fluctuations of the orientation of  $\mathbf{P}$  gives rise to an electric torque  $\mathbf{P} \times \mathbf{E}$  which tends to rotate the particle.
- Stabilization mechanisms: i) The electric field constantly brings new charges to restore the initial dipolar distribution, thereby suppressing the torque. ii) The fluid viscosity opposes the rotation of the particle.

The competition between these mechanisms lead to the existence of a threshold in the applied electric field, under which no rotation occurs. This instability threshold is given by:

$$E_Q = \sqrt{\frac{8}{3} \eta \frac{\sigma_1}{\epsilon_1 \epsilon_s}}, \quad (\text{B1})$$

where  $\eta$  is the dynamic viscosity of the fluid,  $\sigma_1$  its electrical conductivity,  $\epsilon_1$  its permittivity and  $\epsilon_p$  is the particle's permittivity.

Above this threshold, the particle rotate at a constant rate:

$$\Omega = \frac{1}{\tau} \sqrt{\left(\frac{E_0}{E_Q}\right)^2 - 1}, \quad (\text{B2})$$

where  $\tau = \frac{\epsilon_p + 2\epsilon_1}{2\sigma_1}$  is the Maxwell-Wagner relaxation time for the charge distribution at the particle-fluid interface. Note that the rotation rate is independent of the particle size.

#### b. Individual dynamics

The net translation of Quincke-powered colloidal particles follows from their lubricated contact with the lower electrode. Accordingly, the self-propulsion speed reads:

$$v = \zeta a \Omega, \quad (\text{B3})$$

where  $\zeta \in [0, 1]$  quantifies the particle's slip. In our experiments, we measure the self-propulsion speed of both species at low density:  $0.9 \pm 16\% \text{ mm s}^{-1}$  and  $0.7 \pm 16\% \text{ mm s}^{-1}$  for  $10 \mu\text{m}$  and  $7 \mu\text{m}$ , respectively. We note that  $v_\nu/v_\mu \neq a_\nu/a_\mu$ , which reveals (since  $\Omega$  is independent of  $a$ ), that each species experiences different slip, see [3, 4].

Importantly, the Quincke rotation induces the self-propulsion of the colloids without prescribing their direction of motion, which can freely diffuses on the unit circle. An isolated colloidal roller  $i$  performs a persistent random walk governed by its equation of motion:

$$\frac{\partial \mathbf{r}_i}{\partial t} = v \hat{\mathbf{v}}_i \quad (\text{B4})$$

$$\frac{\partial \theta_i}{\partial t} = \sqrt{2Dt}, \quad (\text{B5})$$

where  $\mathbf{r}_i$  is the position of the particle,  $\hat{\mathbf{v}}_i = (\cos \theta_i, \sin \theta_i)$  its direction of motion,  $v$  its self-propulsion speed given by B3, and  $D$  its rotational diffusivity.

#### c. Pairwise interactions

When colloidal rollers are no longer isolated, they experience torques which re-orient their direction of motion. Computing the binary interactions between colloidal rollers proceeds in two steps. First, the response of a roller to perturbations in the hydrodynamics field  $\mathbf{u}_\parallel$  and in the electric field  $\delta \mathbf{E}_\parallel$ , are evaluated. Second, the perturbations in these fields created by a roller in its vicinity are established. Combining both effects, we obtain the pairwise interactions between rollers. This procedure builds on the derivation in [5] for single-component system. In the following sections we refer to particle  $j$  as the particle causing the perturbations and particle  $i$  as the particle responding to these perturbations. Here, we distinguish between the radius of particle  $i$ ,  $a_i$ , and the radius of particle  $j$ ,  $a_j$ , in order to derive both intra- and inter-species interactions by taking all combinations with  $i \in \{\mu, \nu\}$  and  $j \in \{\mu, \nu\}$ .

## 2. Hydrodynamic alignment interactions

### a. Response

A static particle, sitting on a surface whose normal is  $\hat{\mathbf{z}}$ , within a shear flow  $\partial_z \mathbf{u}_{\parallel}$ , experiences a viscous torque  $\mathbf{\Gamma} \propto \hat{\mathbf{z}} \times \partial_z \mathbf{u}_{\parallel}$  which tends to make it rotate. This effect combines with the Quincke electro-rotation mechanism such that colloidal rollers align their direction of motion with the shear according to [5]:

$$\frac{d\theta_i}{dt} = \frac{\tilde{\mu}_s}{\sqrt{\left(\frac{E}{E_Q}\right)^2 - 1}} \hat{\mathbf{v}}_i^{\perp} \cdot \partial_z \mathbf{u}_{\parallel}|_{z=0}, \quad (\text{B6})$$

where  $\tilde{\mu}_s$  is a mobility coefficient and  $\hat{\mathbf{v}}_i^{\perp} = \hat{\mathbf{z}} \times \hat{\mathbf{v}}_i$ . We note that, importantly, the response of particle  $i$  is independent of its size.

### b. Perturbation

A particle rolling on the lower electrode generates a flow in its surrounding. At short distance from the particle, the flow field corresponds to the ones generated by a rotlet close to a non-slip substrate in a semi-infinite medium. At a distance  $\mathbf{r}$  away from particle  $j$  causing this perturbation, the shear reads [5]:

$$\partial_z \mathbf{u}_{\parallel}|_{z=0}(\mathbf{r}) = 6\Omega \frac{a_j^3}{r^3} (\hat{\mathbf{v}}_j \cdot \hat{\mathbf{r}}) \hat{\mathbf{r}} \quad (\text{B7})$$

This flow field is the superposition of a polar field oriented in the direction of  $\hat{\mathbf{v}}_j$  and of a dipolar field similarly oriented, since  $2(\hat{\mathbf{v}}_j \cdot \hat{\mathbf{r}}) \hat{\mathbf{r}} = \hat{\mathbf{v}}_j + (2\hat{\mathbf{r}}\hat{\mathbf{r}} - \mathbf{I}) \hat{\mathbf{v}}_j$ . It is the polar component that is at the origin of alignment interaction between Quincke rollers. Importantly, the amplitude of the flow field generated by a roller is proportional to  $a_j^3$  which quantifies that the larger the colloid, the stronger the hydrodynamic perturbation it causes.

### c. Pairwise alignment

The pairwise alignment interaction between rollers mediated by hydrodynamic is obtained by combining Eqs. B6 and B7. The orientation dynamics reads:

$$\frac{d\theta_i}{dt} = \frac{1}{\tau} \frac{\partial}{\partial \theta_i} \left( 3\tilde{\mu}_s \frac{a_j^3}{r^3} \hat{\mathbf{v}}_i \cdot \hat{\mathbf{v}}_j \right), \quad (\text{B8})$$

where  $r$  is the interparticle distance. This expression establishes the Main text Eq. 2, by defining  $\mathcal{A} = 3\tilde{\mu}_s$ .

## 3. Electrical repulsive interactions

### a. Response

A Quincke roller  $i$  bears a dipole  $\mathbf{P}$ , which makes an angle with the direction of the electric field  $\mathbf{E} = E\hat{\mathbf{z}}$  (see Section B 1 a):  $\mathbf{P} = \mathbf{P}_{\parallel} + P_z \hat{\mathbf{z}}$ . Applying an in-plane electric perturbation  $\delta \mathbf{E}_{\parallel}$  to a roller favors the alignment of  $\mathbf{P}_{\parallel}$  with  $\delta \mathbf{E}_{\parallel}$ . Since the direction of motion  $\hat{\mathbf{v}}_i$  opposes the direction of  $\mathbf{P}_{\parallel}$ , the roller changes its direction of motion to anti-align with  $\delta \mathbf{E}_{\parallel}$  [5]:

$$\frac{d\theta_i}{dt} = -\frac{1}{\tau} \left( \frac{\mu_{\perp}}{\mu_r} - 1 \right) \sqrt{\left(\frac{E}{E_Q}\right)^2 - 1} \hat{\mathbf{v}}_i^{\perp} \cdot \frac{\delta \mathbf{E}_{\parallel}}{E}. \quad (\text{B9})$$

$\mu_r$  and  $\mu_{\perp}$  are mobility coefficients related to the in-plane rotation of the particle and to its rotation around the  $\hat{\mathbf{z}}$ -axis, respectively. We note that the structure of Eq. B9 resembles the structure of Eq. B6 and that, similarly to the hydrodynamic case, the response of particle  $i$  is independent of its size. Unlike the hydrodynamic case, however, the field perturbation  $\delta \mathbf{E}_{\parallel}$  is evaluated at a height  $a_i$  from the lower electrode and might depend on  $a_i$ .

*b. Perturbation*

The perturbation caused by a roller  $j$  to the electric field in its surrounding originates from its dipole  $\mathbf{P}$ . The vertical component  $P_z \hat{\mathbf{z}}$  together with its image through the lower electrode form a dipole  $\mathfrak{P} = 2P_z \mathbf{z}$  centered on the electrode at  $z = 0$ . It gives rise to the perturbation:

$$\delta \mathbf{E}^j(\mathbf{r}) = \frac{3(\mathfrak{P} \cdot \mathbf{r})\mathbf{r} - \mathfrak{P}}{4\pi\epsilon_0 r^3}, \quad (\text{B10})$$

at a distance  $\mathbf{r} = \mathbf{r}_{\parallel} + a\hat{\mathbf{z}}$  from the center of the dipole.  $\epsilon_0$  is the vacuum permittivity. Using the fact that  $\mathfrak{P} \cdot \hat{\mathbf{r}}_{\parallel} = 0$ , the in-plane component reads:

$$\delta \mathbf{E}_{\parallel}^j(\mathbf{r}) = \frac{3}{2\pi\epsilon_0 r_{ij}^3} \left[ \frac{a}{r_{\parallel}} P_z \hat{\mathbf{r}} \right]. \quad (\text{B11})$$

The dipole  $P_z$  is obtained by consideration of the Quincke electro-rotation [5]:

$$P_z = 4\pi\epsilon_0 a_j^3 E \left[ \chi^{\infty} - \left( \chi^{\infty} + \frac{1}{2} \right) \frac{E_Q^2}{E^2} \right], \quad (\text{B12})$$

where  $\chi^{\infty} = (\epsilon_p - \epsilon_l) / (\epsilon_p + 2\epsilon_l)$  is the high frequency polarizability coefficient of the interface. Combining Eqs. B11 and B12 yields the perturbation in the electric field experienced by a roller  $i$  at a distance  $\mathbf{r}$ :

$$\delta \mathbf{E}_{\parallel}^j(\mathbf{r}) = 6E \left[ \chi^{\infty} - \left( \chi^{\infty} + \frac{1}{2} \right) \frac{E_Q^2}{E^2} \right] \frac{a_i a_j^3}{r^4} \hat{\mathbf{r}}. \quad (\text{B13})$$

*c. Pairwise repulsion*

The pairwise repulsion interaction between rollers caused by their Quincke electric dipoles is obtained by combining Eqs. B9 and B13. The orientation dynamics reads:

$$\frac{d\theta_i}{dt} = \frac{1}{\tau} \frac{\partial}{\partial \theta_i} \left\{ 6 \left( \frac{\mu_{\perp}}{\mu_r} - 1 \right) \sqrt{\left( \frac{E}{E_Q} \right)^2 - 1} \left[ \left( \chi^{\infty} + \frac{1}{2} \right) \frac{E_Q^2}{E^2} - \chi^{\infty} \right] \frac{a_i a_j^3}{r^4} \hat{\mathbf{v}}_{\mathbf{i}} \cdot \hat{\mathbf{r}} \right\}, \quad (\text{B14})$$

where  $r$  is the interparticle distance. This expression establishes the Main text Eq. 3, by defining  $\mathcal{B} = 6 \left( \frac{\mu_{\perp}}{\mu_r} - 1 \right) \sqrt{\left( \frac{E_0}{E_Q} \right)^2 - 1} \left[ \left( \chi^{\infty} + \frac{1}{2} \right) \frac{E_Q^2}{E_0^2} - \chi^{\infty} \right]$ .

#### 4. Equations of motions

Considering self-propulsion, rotational diffusion together with alignment and repulsion couplings yields the equations of motion of roller  $i$ :

$$\frac{d\mathbf{r}_{\mathbf{i}}}{dt} = v_i \hat{\mathbf{v}}_{\mathbf{i}}, \quad (\text{B15})$$

$$\frac{d\theta_i}{dt} = \frac{1}{\tau} \frac{\partial}{\partial \theta_i} \sum_j (A_{ij}(r) \hat{\mathbf{v}}_{\mathbf{i}} \cdot \hat{\mathbf{v}}_{\mathbf{j}} + B_{ij}(r) \hat{\mathbf{v}}_{\mathbf{i}} \cdot \hat{\mathbf{r}}) + \sqrt{2D_i} \xi_i(t), \quad (\text{B16})$$

where the sum is over all particles  $j \neq i$ . For binary mixtures, depending on the species  $i$  and  $j$  belong to, the alignment and repulsion torques are given by the corresponding element of the  $2 \times 2$  matrices:

$$\underline{\underline{A}} = \frac{\mathcal{A}}{r^3} \begin{pmatrix} a_{\mu}^3 & a_{\nu}^3 \\ a_{\mu}^3 & a_{\nu}^3 \end{pmatrix}, \quad (\text{B17})$$

and

$$\underline{\underline{B}} = \frac{\mathcal{B}}{r^4} \begin{pmatrix} a_{\mu}^4 & a_{\mu} a_{\nu}^3 \\ a_{\mu}^3 a_{\nu} & a_{\nu}^4 \end{pmatrix}. \quad (\text{B18})$$

This non-reciprocity of interactions complements the heterogeneities of self-propulsion speed and rotational diffusivity.

## Appendix C: Theory: Hydrodynamics of binary mixtures

### 1. Coarse-graining the microscopic dynamics

The hydrodynamic theory is obtained by coarse-graining the microscopic dynamics of Eqs. B15 and B16, following the procedure of [5] for a single-species active liquid. The one-particle distribution function of species  $v \in \{\mu, \nu\}$   $\Psi_v^{(1)}(\mathbf{r}, \theta, t)$  obeys the Fokker-Planck equation:

$$\begin{aligned} & \partial_t \Psi_v^{(1)} + v_v \hat{\mathbf{v}} \cdot \nabla \Psi_v^{(1)} - D_v \partial_\theta^2 \Psi_v^{(1)} \\ & + \frac{1}{\tau} \partial_\theta \int d^2 \mathbf{r}' d\theta' \left( \frac{\partial \mathcal{H}_{v\mu}(\mathbf{r} - \mathbf{r}', \theta, \theta')}{\partial \theta} \Psi_{v\mu}^{(2)}(\mathbf{r}, \mathbf{r}', \theta, \theta', t) + \frac{\partial \mathcal{H}_{v\nu}(\mathbf{r} - \mathbf{r}', \theta, \theta')}{\partial \theta} \Psi_{v\nu}^{(2)}(\mathbf{r}, \mathbf{r}', \theta, \theta', t) \right) = 0. \end{aligned} \quad (\text{C1})$$

where the effective potentials  $\mathcal{H}_{v\mu}$  and  $\mathcal{H}_{v\nu}$  are given by:

$$\mathcal{H}_{v\gamma}(\mathbf{r}, \hat{\mathbf{v}}_i, \hat{\mathbf{v}}_j) = \sum_{j \in \gamma} A_{ij}(r) \hat{\mathbf{v}}_i \cdot \hat{\mathbf{v}}_j + B_{ij}(r) \hat{\mathbf{v}}_i \cdot \hat{\mathbf{r}}, \quad (\text{C2})$$

with  $\gamma \in \{\mu, \nu\}$ . We assume no two-body correlations outside of hard-core exclusion, such that the two-point distribution functions satisfy:

$$\Psi_{v\gamma}^{(2)}(\mathbf{r}, \mathbf{r}', \theta, \theta', t) = 0, \quad \text{if } |\mathbf{r} - \mathbf{r}'| < a_v + a_\gamma, \quad (\text{C3})$$

$$\Psi_{v\gamma}^{(2)}(\mathbf{r}, \mathbf{r}', \theta, \theta', t) = \Psi_v^{(1)}(\mathbf{r}, \theta, t) \Psi_\gamma^{(1)}(\mathbf{r}', \theta', t), \quad \text{if } |\mathbf{r} - \mathbf{r}'| \geq a_v + a_\gamma. \quad (\text{C4})$$

The density fields  $\rho_v$ , the polarization fields  $\mathbf{\Pi}_v$  and the nematic tensor field  $\underline{\underline{\mathbf{Q}}}_v$  are defined, for  $v \in \{\mu, \nu\}$  as:

$$\rho_v(\mathbf{r}, t) = \int d\theta \Psi_v^{(1)}(\mathbf{r}, \theta, t), \quad (\text{C5})$$

$$\mathbf{\Pi}_v(\mathbf{r}, t) = \frac{1}{\rho} \int d\theta \hat{\mathbf{v}} \Psi_v^{(1)}(\mathbf{r}, \theta, t), \quad (\text{C6})$$

$$\underline{\underline{\mathbf{Q}}}_v(\mathbf{r}, t) = \frac{1}{\rho} \int d\theta \left( \hat{\mathbf{v}} \hat{\mathbf{v}} - \frac{1}{2} \mathbf{I} \right) \Psi_v^{(1)}(\mathbf{r}, \theta, t). \quad (\text{C7})$$

Integrating Eq. C2 over  $\theta$  results in the mass conservation equation of each species:

$$\partial_t \rho_v + v_v \nabla \cdot (\rho \mathbf{\Pi}_v) = 0, \quad (\text{C8})$$

which corresponds to the Main text Eq. 4.

### 2. Evolution equation for the polarization

The evolution equation for the polarization field  $\mathbf{\Pi}_v$  is obtained by multiplying Eq. C2 by  $\hat{\mathbf{v}}$  and integrating over  $\theta$ . We simplify the notation  $\Psi_v^{(1)} \equiv \Psi_v$  and treat each term of Eq. C2 separately.

- The rotational diffusion term gives:

$$\int_0^{2\pi} d\theta D_v \partial_\theta^2 \Psi_v \hat{\mathbf{v}} = -D_v \rho_v \mathbf{\Pi}_v. \quad (\text{C9})$$

- The self-propulsion gives the convection contribution:

$$\int_0^{2\pi} d\theta v_v (\hat{\mathbf{v}} \cdot \nabla) \Psi_v \hat{\mathbf{v}} = v_v \nabla \cdot \left[ \rho_v \underline{\underline{\mathbf{Q}}}_v + \frac{\rho_v}{2} \mathbf{I} \right]. \quad (\text{C10})$$

- The alignment caused by the species  $\gamma \in \{\mu, \nu\}$  contributes through:

$$\begin{aligned} & \int_0^{2\pi} d\theta \frac{1}{\tau} \partial_\theta \left\{ \Psi_v(\mathbf{r}, \theta) \int_{|\mathbf{r}-\mathbf{r}'| \geq a_v + a_\gamma} \partial_\theta (A_{v\gamma}(|\mathbf{r}-\mathbf{r}'|) \hat{\mathbf{v}}' \cdot \hat{\mathbf{v}}) \Psi_\gamma(\mathbf{r}', \theta') d\mathbf{r}' d\theta' \right\} \hat{\mathbf{v}} \\ &= \frac{\rho_v}{\tau} \left( \frac{\mathbf{I}}{2} - \underline{\underline{\mathbf{Q}_v}} \right) \left( \int_{|\mathbf{u}| \geq a_v + a_\gamma} A_{v\gamma}(|\mathbf{u}|) (\rho_\gamma \mathbf{\Pi}_\gamma)_{|\mathbf{r}-\mathbf{u}} d\mathbf{u} \right) \\ &\simeq \rho_v \left( \mathbf{I} - 2\underline{\underline{\mathbf{Q}_v}} \right) (\alpha_{v\gamma} \rho_\gamma \mathbf{\Pi}_\gamma), \end{aligned} \quad (\text{C11})$$

where the last approximation follows from keeping the zeroth-order term in a Taylor expansion defining the hydrodynamic alignment coefficient:

$$\alpha_{v\gamma} = \frac{1}{2\tau} \int_{|\mathbf{u}| > a_v + a_\gamma} A_{v\gamma}(|\mathbf{u}|) d\mathbf{u} = \mathcal{A} \frac{\pi}{\tau} \frac{a_\gamma^3}{a_v + a_\gamma}. \quad (\text{C12})$$

- The repulsion caused by the species  $\gamma \in \{\mu, \nu\}$  contributes through:

$$\begin{aligned} & \int_0^{2\pi} d\theta \frac{1}{\tau} \partial_\theta \left\{ -\Psi_v(\mathbf{r}, \theta) \int_{|\mathbf{r}-\mathbf{r}'| \geq a_v + a_\gamma} \partial_\theta \left( B_{v\gamma}(|\mathbf{r}-\mathbf{r}'|) \frac{\mathbf{r}-\mathbf{r}'}{|\mathbf{r}-\mathbf{r}'|} \cdot \hat{\mathbf{v}} \right) \Psi_\gamma(\mathbf{r}', \theta') d\mathbf{r}' d\theta' \right\} \hat{\mathbf{v}} \\ &= -\frac{\rho_v}{\tau} \left( \frac{\mathbf{I}}{2} - \underline{\underline{\mathbf{Q}_v}} \right) \left( \int_{|\mathbf{u}| \geq a_v + a_\gamma} B_{v\gamma}(|\mathbf{u}|) \frac{\mathbf{u}}{|\mathbf{u}|} (\rho'_\gamma)_{|\mathbf{r}-\mathbf{u}} d\mathbf{u} \right) \\ &\simeq -\rho_v \left( \mathbf{I} - 2\underline{\underline{\mathbf{Q}_v}} \right) (\beta_{v\gamma} \nabla \rho_\gamma) \end{aligned} \quad (\text{C13})$$

where the last approximation follows from keeping the first-order term in a Taylor expansion defining the hydrodynamic repulsion coefficient:

$$\beta_{v\gamma} = \frac{1}{2\tau} \int_{|\mathbf{u}| > a_v + a_\gamma} B_{v\gamma}(|\mathbf{u}|) \frac{|\mathbf{u}|^2}{|\mathbf{u}|} d\mathbf{u} = \mathcal{B} \frac{\pi}{\tau} \frac{a_\gamma^3 a_v}{a_v + a_\gamma}. \quad (\text{C14})$$

The momentum evolution equation for species  $v \in \{\mu, \nu\}$  is obtained by combining the various contributions evaluated above:

$$\partial_t(\rho_v \mathbf{\Pi}_v) + v_v \nabla \cdot \left( \rho_v \underline{\underline{\mathbf{Q}_v}} + \frac{\rho_v}{2} \mathbf{I} \right) = -D_v \rho_v \mathbf{\Pi}_v + \rho_v \left( \mathbf{I} - 2\underline{\underline{\mathbf{Q}_v}} \right) \sum_{\gamma \in \{\mu, \nu\}} (\alpha_{v\gamma} \rho_\gamma \mathbf{\Pi}_\gamma - \beta_{v\gamma} \nabla \rho_\gamma), \quad (\text{C15})$$

which corresponds to the Main text Eq. 5.

By coarse-graining the microscopic equations of motions of colloidal rollers of two species  $\mu$  and  $\nu$  interacting through hydrodynamic alignment coupling and electric repulsive coupling, we have established the Toner-Tu hydrodynamic equations for their binary mixtures Eqs. C8 and C15. At the hydrodynamic levels, distinct coefficients account for alignment and repulsion interaction intra- and inter-species. Evaluating these coefficients from microscopic parameters (Eqs. C12 and C14) gives:

$$\underline{\underline{\alpha}} = \alpha_{\mu\mu} \begin{pmatrix} 1 & 0.40 \\ 1.18 & 0.49 \end{pmatrix}, \quad (\text{C16})$$

and

$$\underline{\underline{\beta}} = \beta_{\mu\mu} \begin{pmatrix} 1 & 0.40 \\ 0.82 & 0.34 \end{pmatrix}, \quad (\text{C17})$$

where  $\alpha_{\mu\mu} = 3.2 \times 10^4 \mu\text{m}^2/\text{s}$  and  $\beta_{\mu\mu} = 1.3 \times 10^5 \mu\text{m}^3/\text{s}$ . Note that these estimations from first principles are in remarkable agreement with the values determined experimentally, see Eq. 6 and below.

### 3. Hydrodynamic equations in polar geometry

To establish the radial density profiles of species  $\mu$  and  $\nu$ , we look for axisymmetric stationary solutions of Eqs. C8 and C15, extending to binary mixtures the single-species case of [6].

Using standard polar coordinates  $(r, \varphi)$ , the density, polarization and nematic fields read:

$$\rho_v = \rho_v(r), \quad (C18)$$

$$\mathbf{\Pi}_v = \Pi_v(r) \hat{\mathbf{e}}_\varphi, \quad (C19)$$

$$\underline{\underline{\mathbf{Q}}}_v = Q_v(r) (\hat{\mathbf{e}}_\varphi \hat{\mathbf{e}}_\varphi - \hat{\mathbf{e}}_r \hat{\mathbf{e}}_r), \quad (C20)$$

for  $v \in \{\mu, \nu\}$ .

Projecting Eq. C15 onto the azimuthal direction  $\hat{\mathbf{e}}_\varphi$  yields:

$$-D_\mu \rho_\mu \Pi_\mu + \rho_\mu (1 - 2Q_\mu) [\alpha_{\mu\mu} \rho_\mu \Pi_\mu + \alpha_{\mu\nu} \rho_\nu \Pi_\nu] = 0, \quad (C21)$$

while its projection onto the radial direction  $\hat{\mathbf{e}}_r$  yields:

$$v_\mu \left[ \left( \frac{\partial(-\rho_\mu Q_\mu)}{\partial r} + \frac{1}{2} \frac{\partial \rho_\mu}{\partial r} \right) - \frac{2\rho_\mu Q_\mu}{r} \right] = -\rho_\mu (1 + 2Q_\mu) \left( \beta_{\mu\mu} \frac{\partial \rho_\mu}{\partial r} + \beta_{\mu\nu} \frac{\partial \rho_\nu}{\partial r} \right). \quad (C22)$$

We see that contributions from rotational diffusion and alignment balance each other in Eq. C21, while convection and repulsion compete in Eq. C22. Similar equations are obtained from the momentum evolution of species  $\nu$  by inverting the subscripts  $\mu \leftrightarrow \nu$ . In what follows, we proceed in solving Eqs. C21 and C22 in two different ways, each highlighting a different route for the spontaneous demixing of the binary polar liquid, as discussed in the Main text. First, we consider the case of colloidal flocks, for which self-propulsion speed heterogeneity is crucial in the demixing. Second, we consider a situation where non-reciprocity of the repulsion interactions drives the demixing.

### 4. Hydrodynamics of colloidal flocks

In order to establish the radial density profiles for the 10  $\mu\text{m}$ – and 7  $\mu\text{m}$ –diameter colloidal rollers, we consider the following simplifications based on experimental evidence.

First, we notice that the polarization of both species are very close to each other at any location within the binary vortex. As an example, Fig. 6 shows the radial polarization profiles corresponding to the density profiles of the Main text Fig. 1(c). Therefore, we take  $\Pi_\mu(r) = \Pi_\nu(r)$ .

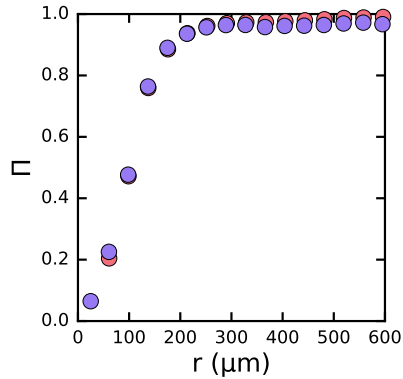

FIG. 6. Radial profiles of the polarization for the 52:48 binary colloidal flock of 10  $\mu\text{m}$  particles (red), and 7  $\mu\text{m}$  particles (violet). These polarization profiles correspond to the density profiles of the Main text Fig. 1(c).

Second, we need a closure relation specifying the nematic fields. We find that the closure relation  $Q(r) = \Pi^2(r)/2$ , which amounts to neglecting correlations in polarization [6], describes very well the experimental measurements, see Fig. 7.

Third, we use the structure of Eqs. 6, such that only two coefficients relate to the non-reciprocal alignment interactions and two coefficients relate to the non-reciprocal repulsion interactions:

$$\underline{\underline{\alpha}} = \begin{pmatrix} \alpha_{\mu\mu} & \alpha_{\nu\nu} \\ \alpha_{\mu\nu} & \alpha_{\nu\mu} \end{pmatrix}, \quad \underline{\underline{\beta}} = \begin{pmatrix} \beta_{\mu\mu} & \beta_{\nu\nu} \\ \beta_{\mu\nu} & \beta_{\nu\mu} \end{pmatrix}. \quad (C23)$$

The experimental determination of these coefficients is detailed in Section D.

Altogether, these simplifications make the projection of the momentum dynamics on the azimuthal direction straightforwardly solvable for the polarization field, which reads:

$$\Pi(r) = \sqrt{1 - \frac{D}{\alpha_{\mu\mu}\rho_\mu(r) + \alpha_{\nu\nu}\rho_\nu(r)}}, \quad (\text{C24})$$

where, for consistency, the rotational diffusion coefficients  $D_\mu$  and  $D_\nu$  are assimilated to a single coefficient  $D = (N_\mu D_\mu + N_\nu D_\nu) / N_{\mu+\nu}$ . This expression is very similar to the single-component case and expresses that the local polarization is set by the competition between orientational noise and the alignment strength, proportional to the local density.

Most interesting for the demixing of the binary flocks is the projection on the radial direction. Combining judiciously the two equations Eq. C22 for species  $\mu$  and  $\nu$ , yields:

$$\frac{2Q}{r} \frac{v_\mu v_\nu}{v_\mu \chi_\nu^a + v_\nu \chi_\mu^a} = (1 + 2Q) \beta_{\mu\mu} \frac{\partial \rho^b}{\partial r}, \quad (\text{C25})$$

$$2\alpha_{\mu\mu}\beta_{\mu\mu} \frac{v_\mu - v_\nu}{v_\mu v_\nu} \rho^a (1 + 2Q) \frac{\partial \rho^b}{\partial r} = \frac{D}{\chi_\mu^a \chi_\nu^a} \frac{\partial \chi_\mu^a}{\partial r}, \quad (\text{C26})$$

where we have introduced the shorthand notations  $\rho^b = \rho_\mu + b\rho_\nu$ ,  $\rho^a = \rho_\mu + a\rho_\nu$ ,  $\chi_\mu^a = \rho_\mu / (\rho_\mu + a\rho_\nu)$  and  $\chi_\nu^a = a\rho_\nu / (\rho_\mu + a\rho_\nu)$ . In these expressions,  $a$  and  $b$  quantifies the non-reciprocity of alignment and repulsion interactions:  $a = \alpha_{\mu\nu} / \alpha_{\mu\mu}$  and  $b = \beta_{\mu\nu} / \beta_{\mu\mu}$  respectively. Equations C25 and C26 reduce to the Main text Eqs. 7 and 8 when non-reciprocity is ignored ( $a = 1$ , and  $b = 1$ ). In the more general case of  $a \neq 1$  and  $b \neq 1$ , non-reciprocity plays an intricate role. The structure of Eqs. C25 and C26 does remain similar: Eq. C25 predicts the monotonous increase of  $\rho^b$ , and Eq. C26 relates the self-propulsion speed difference to the gradient of  $\chi^a$ . Despite that  $a \approx 1/2$  for colloidal flock, the opposite monotonous behaviours for species  $\mu$  and  $\nu$  is preserved and matches the experimental observations.

Equation C26 can be integrated:

$$2\alpha_{\mu\mu}\beta_{\mu\mu} \left( \frac{v_\mu - v_\nu}{v_\mu v_\nu} \right) \left[ \left( 1 - \frac{b}{a} \right) \left( 3\rho^a - \frac{2D}{\alpha_{\mu\mu}} \right) \rho^a \chi_\mu^a + \frac{b}{a} \rho^a \left( \rho^a - \frac{D}{\alpha_{\mu\mu}} \right) \right] = D \log \left( C \frac{\chi_\mu^a}{1 - \chi_\mu^a} \right), \quad (\text{C27})$$

where  $C$  is an integration constant.

The theoretical density profiles are obtained by numerically solving the differential equation Eq. C25 and Eq. C27 on a discrete grid of spacing  $\delta r = 5 \mu\text{m}$ . The solving procedure is as follow. Starting from  $\chi_\mu^a(r) = \chi_\nu^a(r) = 0.5$ , Eq. C25 is integrated to obtain the density profiles (step (i)), with the integration constant determined by imposing the overall particle density. Next, the particle fraction  $\chi_\mu^a(r)$  is evaluated from Eq. C27 (step (ii)): the secant method is used to adjust the value of the integration constant  $C$  until the total density of each species is respected. The above procedure (steps (i) and (ii)) is repeated until the particle fraction converges: the relative difference between

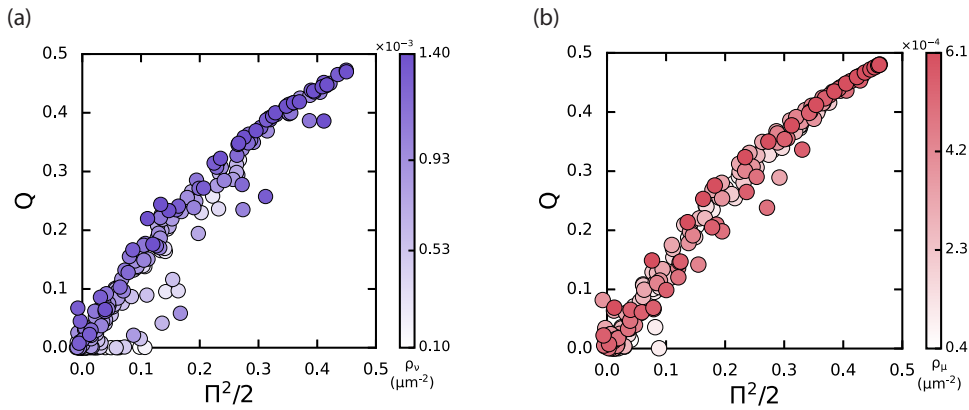

FIG. 7. Experimental validation of the closure relation  $Q(r) = \Pi^2(r)/2$ . Scatter plot of the  $Q$  versus  $\Pi^2/2$  for single-components colloidal flocks confined within 2.1 mm-diameter wells. (a)  $7 \mu\text{m}$ -diameter particles (b)  $10 \mu\text{m}$ -diameter particles. The colorbars indicate the total particle density particle densities which range from just beyond the flocking threshold  $\rho^*$  up to about  $13 \rho^*$ .

subsequent estimations of  $\chi^a$  becomes less than 2%. In practice, step (i) is implemented using Scipy Initial Value Problem solver, using an initial value of  $\rho^a(r=0) = 1.001D/\alpha_{\mu\mu}$  to force a positive value of  $\Pi$ , see Eq. C24 needed for numerical convergence. The final solution is independent of this choice.

Following the procedure above allows to establish the radial density profiles of both species, without any fitting parameter. Figure 8 shows the profiles obtained for the 52 : 48 binary mixture of the Main text Fig. 1(c). As discussed in the Main text, three different cases are considered:

- i) keeping both the self-propulsion speed heterogeneity and the interaction non-reciprocity,
- ii) keeping only the self-propulsion speed heterogeneity,
- iii) keeping only the non-reciprocity of interactions.

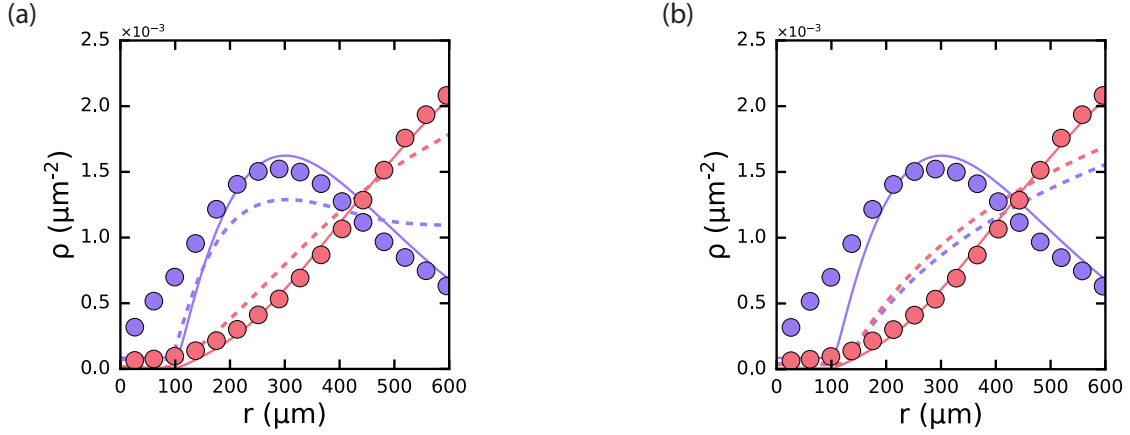

FIG. 8. Radial density profiles. Experimental data (markers), case i) (solid lines), case ii) (dashed line in panel (a)), and case iii) (dashed line in panel (b)). Excellent quantitative agreement is obtained when both difference in self-propulsion speeds and non-reciprocity of the interactions are taken into account.

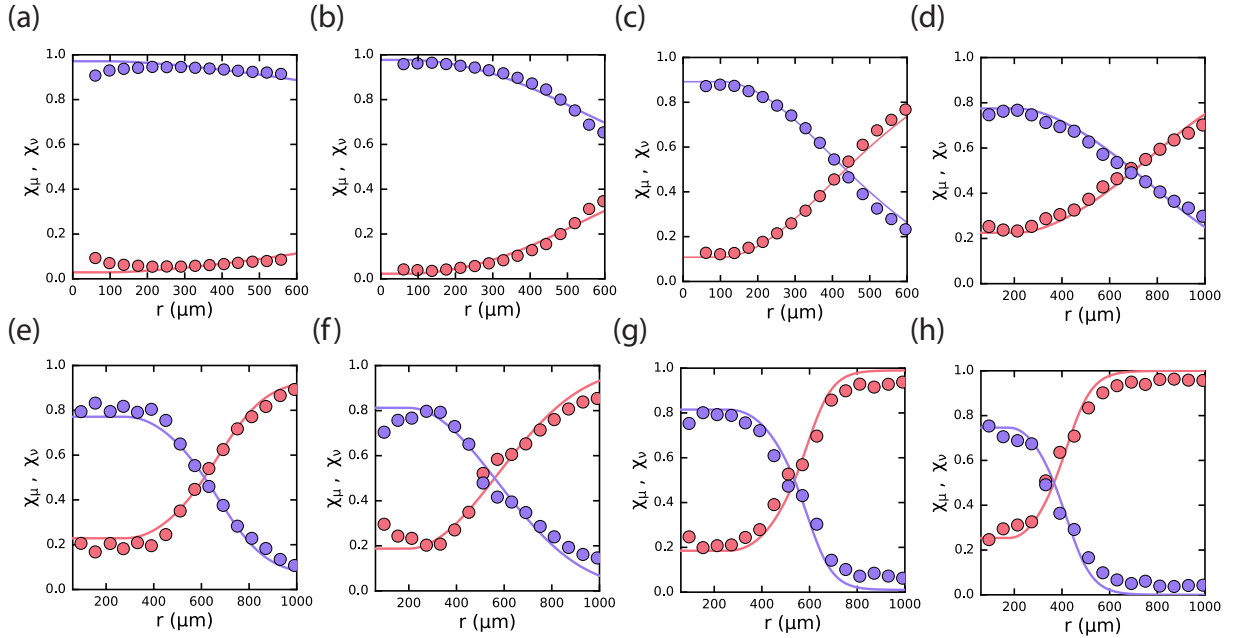

FIG. 9. Density fraction profiles at steady-state for binary flocks of different mixtures corresponding to Fig. 5. Confinement size:  $d = 1.2$  mm (a)-(c),  $d = 2.1$  mm (d)-(h). Violet:  $7 \mu\text{m}$ -diameter colloidal particles. Red:  $10 \mu\text{m}$ -diameter colloidal particles. Markers: experimental data. Lines: theory.

Figure 9 shows that the excellent agreement obtained between theory and experiments extends to mixtures of

different ratios. It is noteworthy that the profiles of the particle fractions show an even better match than the corresponding density profiles reported in Fig. 5, especially towards the core of the polar vortex ( $r \in [0, 200] \mu\text{m}$ ). The underlying reason is that the particle fraction at the core is not locally dependent on the total density, but is set by the integration constant  $C$  from Eq. C27 (obtained by enforcing the conservation of the total number of particles of each species). Indeed, at low  $r$ , the left-hand side of Eq. C27 is negligible in comparison to the right-hand side.

### 5. Non-reciprocity driven demixing

To highlight how non-reciprocal interactions can lead to the spontaneous demixing of binary polar liquids, we proceed with the hydrodynamics description of Section C3, without the constraints of the interaction rules obeyed by colloidal rollers. In place, we make the following simplifications:

First, we consider species with identical rotational diffusivities and self-propulsion speeds:  $D_\mu = D_\nu$ ,  $v_\mu = v_\nu$ , later referred to as  $D$  and  $v$ , respectively.

Second, we close the system of equations with  $Q_\mu = \Pi_\mu^2/2$  and  $Q_\nu = \Pi_\nu^2/2$ .

Third, we consider a situation where species  $\mu$  is insensitive to species  $\nu$ : it behaves exactly as in a single-component flock. Within this active background, species  $\nu$  evolves, only experiencing heterospecific interactions. The statistically-averaged behaviour of species  $\nu$  is therefore independent of its total density. This situation, which echoes leader/follower dynamics, is summarized by the interaction rules:

$$\underline{\alpha} = \begin{pmatrix} \alpha_{\mu\mu} & 0 \\ \alpha_{\mu\mu} & 0 \end{pmatrix}, \quad \underline{\beta} = \begin{pmatrix} \beta_{\mu\mu} & 0 \\ \beta_{\nu\mu} & 0 \end{pmatrix}, \quad (\text{C28})$$

where for simplicity we have also taken  $\alpha_{\nu\mu} = \alpha_{\mu\mu}$ , later referred to as  $\alpha$ .

The density and polarization profiles of species  $\mu$  are given by the single-component solution [6]. The density profile is obtained from the radial projection of the momentum dynamics. It is given by the implicit relation:

$$\frac{r}{r^*} = \exp \left[ 2 \frac{\beta_{\mu\mu}}{v} \rho_\mu(r) + \rho^* \frac{\beta_{\mu\mu}}{v} \ln \left( \frac{\rho_\mu(r)}{\rho^*} - 1 \right) \right]. \quad (\text{C29})$$

where  $\rho^* = D/\alpha$  is the flocking density threshold and  $r^*$  is an integration constant determined through mass conservation. The polarization profile follows from the azimuthal projection of the momentum dynamic. It is locally slaved to the density through:

$$\Pi(r) = \sqrt{1 - \frac{\rho^*}{\rho(r)}}. \quad (\text{C30})$$

The polarization profiles of species  $\nu$  follows similarly from the azimuthal projection and reads:

$$\Pi_\nu(r) = \sqrt{1 + \left( \frac{D}{4\alpha\rho_\mu\Pi_\mu} \right)} - \frac{D}{2\alpha\rho_\mu\Pi_\mu} \simeq 1 - \frac{3}{8} \frac{D}{\alpha\rho_\mu(r)\Pi_\mu(r)}, \quad (\text{C31})$$

where the last approximation is valid at first order.

Working out the radial projection, the density profile  $\rho_\nu(r)$  can be expressed in terms of the density and polarization fields of species  $\mu$ :

$$\rho_\nu(r) = \rho_\mu(r) \frac{\rho_\nu(r_0)}{\rho_\mu(r_0)} \exp \left[ \int_{r_0}^r \mathcal{C}(r') - \mathcal{R}(r') dr' \right], \quad (\text{C32})$$

where

$$\mathcal{C}(r) = 2 \frac{\rho_\mu}{\rho^*} \Pi_\mu \frac{\Pi_\nu}{r}, \quad (\text{C33})$$

$$\mathcal{R}(r) = 2\beta_{\nu\mu} \frac{\rho_\mu}{v\rho^*} (1 + \Pi_\nu^2) \frac{\partial \rho_\mu}{\partial r}, \quad (\text{C34})$$

and  $r_0$  is an arbitrary position along the radial direction. Beyond its apparent complexity, Eq. C32 expresses the competition between an effective centrifuge effect  $\mathcal{C}$  and repulsion  $\mathcal{R}$ . Taking  $r_0$  where the density ratio  $\rho_\nu(r)/\rho_\mu(r)$  is maximal, this ratio will decrease for  $r > r_0$  when the repulsion dominates the centrifuge effect  $\mathcal{R}(r_0) > \mathcal{C}(r_0)$ . Note, however, that this competition acts in a non-local fashion. The key parameter which controls the density profile of species  $\nu$  is  $\beta_{\nu\mu}$  which characterizes the repulsion they experience from species  $\mu$ . As shown in Fig. 10 and discussed in the Main text (Fig. 4(b)), varying the ratio  $\beta_{\nu\mu}/\beta_{\mu\mu}$  controls the spontaneous demixing of the binary flock.

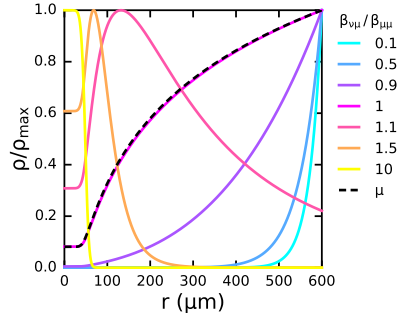

FIG. 10. Non-reciprocity driven demixing. The radial density profiles of species  $\nu$  (solid lines) show accumulation towards the confinement edge for  $\beta_{\nu\mu} > \beta_{\mu\mu}$  and towards the core for  $\beta_{\nu\mu} < \beta_{\mu\mu}$ . The density profile of species  $\mu$  (dashed black line) remains unchanged, and correspond to the single-component polar liquid given by Eq. C29. The density profiles are normalized by their maximal value. The values of the parameters are:  $v = 1 \text{ mm/s}$ ,  $\rho^* = 100 \text{ mm}^{-2}$ ,  $\langle \rho_\mu(\mathbf{r}) \rangle_{\mathbf{r}} = 10\rho^*$ , as in the Main text Fig. 4(b).

#### Appendix D: Experiments: Measurements of the hydrodynamic coefficients

In this section, we detail the experimental evaluation of the alignment and repulsion coefficients  $\underline{\alpha}$  and  $\underline{\beta}$ , reported in the Main text Eq. 6.

##### 1. Alignment interactions

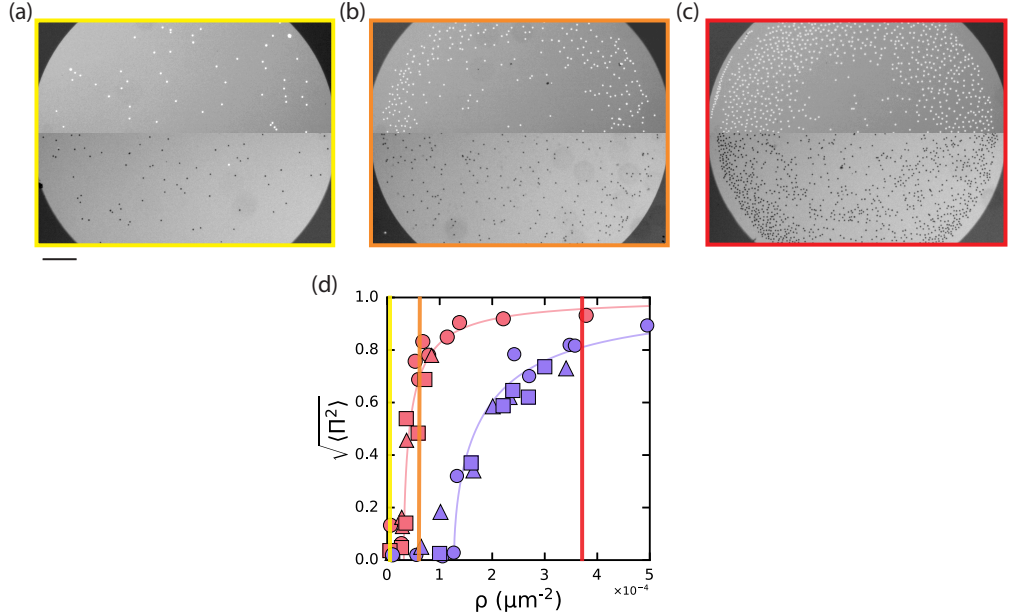

FIG. 11. Determination of the flocking threshold. (a)-(c) Colloidal rollers confined within circular wells at various densities. Top panels: fluorescent  $10 \mu\text{m}$ - diameter colloids. Bottom panels: non-fluorescent  $7 \mu\text{m}$ - diameter colloids. The larger colloidal rollers flock at a lower density than the smaller ones. Scale bar:  $250 \mu\text{m}$ . (d) Variations of the system polarization with density, whose bifurcation indicates the flocking transition. The theoretical fit Eq. D1 gives:  $\rho_\mu^* = 3.6 \times 10^{-5} \mu\text{m}^{-2}$  for the  $10 \mu\text{m}$  particles (red), and  $\rho_\nu^* = 13.2 \times 10^{-5} \mu\text{m}^{-2}$  for the  $7 \mu\text{m}$  particles (violet). The diameter of the confinement wells is  $2.1 \text{ mm}$  for circles,  $4.2 \text{ mm}$  for triangles, and  $8.4 \text{ mm}$  for squares. The vertical lines indicate the density represented in panels (a)-(c).

The diagonal components of  $\underline{\alpha}$ ,  $\alpha_{\mu\mu}$  and  $\alpha_{\nu\nu}$ , are measured by performing experiments on single-component colloidal flocks of various density  $\langle \rho_v(\mathbf{r}) \rangle_{\mathbf{r}}$ , with  $v \in \{\mu, \nu\}$ , see Fig. 11. For single component flock, the alignment coefficient

is given by the ratio of the rotational diffusivity and the threshold density of flocking:  $\alpha_{vv} = D_v/\rho_v^*$ .  $D_v$  is measured as described in Section A 1.  $\rho_v^*$  is obtained from the bifurcation of the flock polarization at the transition, derived from Eq. C30:

$$\sqrt{\langle \Pi_v^2 \rangle} = \sqrt{1 - \frac{\rho_v^*}{\langle \rho_v(\mathbf{r}) \rangle_{\mathbf{r}}}}, \quad (\text{D1})$$

where  $\langle \Pi_v^2 \rangle = \int \Pi^2(\mathbf{r})\rho(\mathbf{r})d\mathbf{r} / \int \rho(\mathbf{r})d\mathbf{r}$ . Our experiment reveals that 10  $\mu\text{m}$ -diameter colloidal rollers flock at a much lower density than the 7  $\mu\text{m}$ -diameter ones as shown in Fig. 11. Furthermore, the flocking threshold is independent of the confinement size.

To determine the off-diagonal coefficients of  $\underline{\underline{\alpha}}$ , we perform experiments to measure the response of colloidal rollers to hydrodynamic fields imposed externally, see Eq. B6. The experimental protocol is similar to the one described in [7]. An external hydrodynamic field is realized by flowing solvent at a controlled rate through the microfluidic device filled with a dilute mixture of particles. As illustrated in Fig. 12(a), the rollers reorient to align their direction of motion with the external flow field. Rotational diffusion, however, prevents perfect alignment. This competition yields the increase of the average polarization such that, for  $u_{\parallel} \rightarrow 0$ :

$$\langle \Pi \rangle \sim \frac{\tilde{\mu}_s}{2\sqrt{\left(\frac{E}{E_Q}\right)^2 - 1}} \frac{\partial_z u_{\parallel}}{D}. \quad (\text{D2})$$

We validate this evolution experimentally in Fig. 12(b) for both species and confirms that the response to the hydrodynamic field is independent of the particle size. Consequently, we can identify  $\alpha_{\nu\mu}$  with  $\alpha_{\mu\mu}$ , and  $\alpha_{\mu\nu}$  with  $\alpha_{\mu\mu}$ .

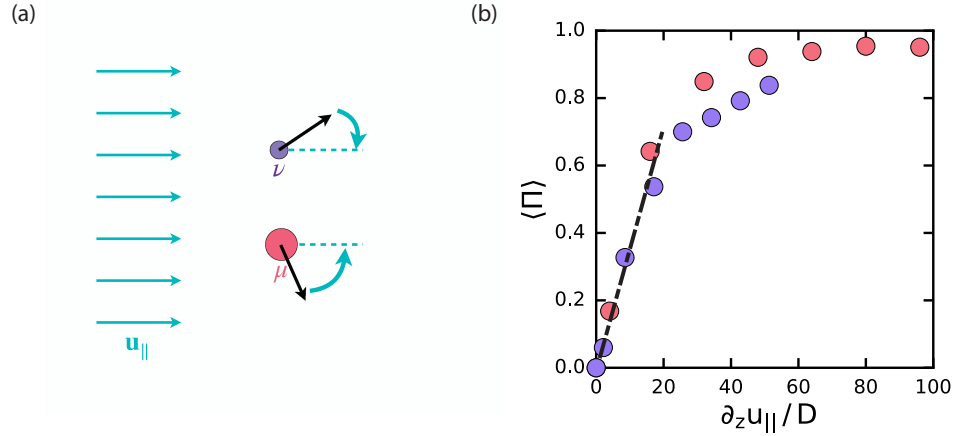

FIG. 12. (a) Schematic of the reorientation of the two roller species under the influence of an externally applied hydrodynamic field. The hydrodynamic perturbation  $u_{\parallel}$  is created by the controlled injection of the fluids surrounding the rollers within the microfluidic device, see Methods in Section A 1. (b) Polarization of colloidal rollers of both species within a dilute mixture under varying strength of hydrodynamic shear  $\partial u_{\parallel} / \partial z$ , normalized by the rotational diffusion  $D$ . At low shear, both species show the same response as predicted by Eq. D2

Overall, these two sets of experiments allow us to infer the alignment coefficients entering the Toner-Tu like equation Eq. C15:

$$\underline{\underline{\alpha}} = 5.5 \times 10^4 \begin{bmatrix} 1 & 0.53 \\ 1 & 0.53 \end{bmatrix} \mu\text{m}^2/\text{s}. \quad (\text{D3})$$

## 2. Repulsive interactions

The diagonal components of  $\beta$ ,  $\beta_{\mu\mu}$  and  $\beta_{\nu\nu}$ , are measured experimentally on single-species flocks. Specifically, the radial density profile, given by Eq. C29, increases logarithmically at large  $r$  as

$$\rho_v(r) \sim \frac{v_v}{2\beta_{vv}} \ln(r), \quad (\text{D4})$$

as shown in Fig. 13(a). Figure 13(b) shows unambiguously that  $\beta_{\mu\mu} > \beta_{\nu\nu}$ .

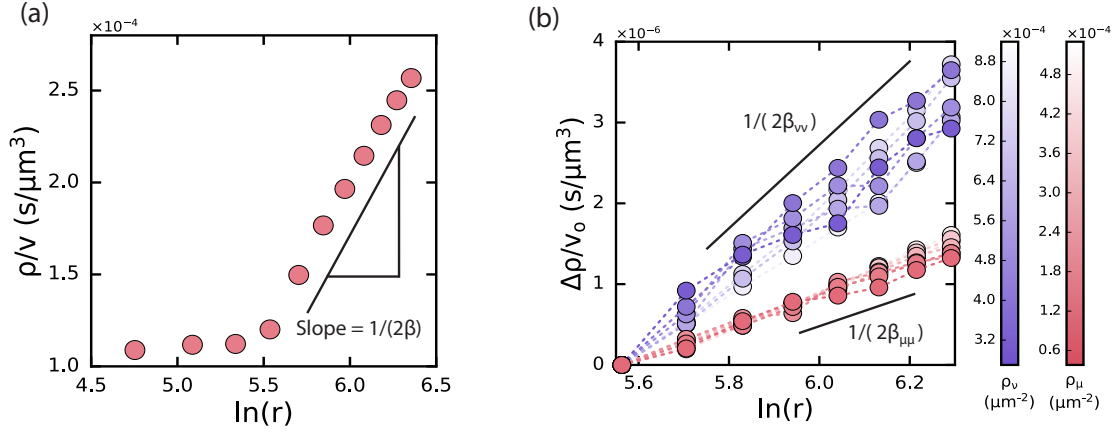

FIG. 13. Determination of the homospecific repulsive interaction strengths. (a) Density profile of a single-component flock assembled from  $10\text{ }\mu\text{m}$ -diameter colloidal particles. At large  $r$ , the density increases logarithmically, see Eq. D4. Average density indicated by the color in (b). (b) Density profiles of single-species colloidal flocks of various average densities  $\langle\rho_\mu(\mathbf{r})\rangle_r$  (red) and  $\langle\rho_\nu(\mathbf{r})\rangle_r$  (violet). The profiles are shifted by  $\rho_\nu(r = 250\text{ }\mu\text{m})$  for easier visual comparison.

To determine the off-diagonal coefficients of  $\underline{\beta}$ , we perform experiments to measure the response of colloidal rollers of both species  $\mu$  and  $\nu$  to a perturbation in the electric fields caused by a static particle of  $10\text{ }\mu\text{m}$  diameter. As depicted in Fig. 14(a), the direction of motion of colloidal rollers is deflected upon collision with the static particle, from  $\hat{\mathbf{v}}_{\text{in}}$  to  $\hat{\mathbf{v}}_{\text{out}}$ . We quantify this repulsive interaction by measuring the scattering angle  $\delta\theta$  as a function of the impact parameter  $B$ , defined as:

$$B = (\mathbf{r}_{\text{in}} \times \hat{\mathbf{v}}_{\text{in}}) \cdot \hat{\mathbf{z}}. \quad (\text{D5})$$

Figure 14(b) shows that the scattering dynamic of both species are sensibly identical. The difference predicted by Eq. B18 can not be confirmed experimentally. Consequently, we identify  $\beta_{\nu\mu}$  with  $\beta_{\mu\mu}$ , and  $\beta_{\mu\nu}$  with  $\beta_{\mu\mu}$ .

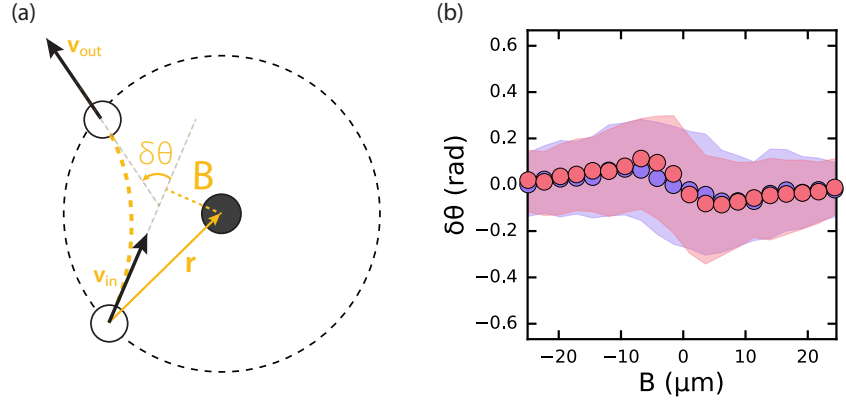

FIG. 14. (a) Schematic of the re-orientation of a colloidal roller  $v \in \{\mu, \nu\}$  (white disk) upon scattering on a static  $10\text{ }\mu\text{m}$ -diameter particle (black disk). (b) Variation of the scattering angle  $\delta\theta$  with the impact parameter  $B$ . The repulsive strengths experienced by both species are similar. The radius of the interaction window (dashed circle) is  $25\text{ }\mu\text{m}$ . For each species, about  $10^4$  collisions are monitored.

Overall, these two sets of experiments allow us to infer the repulsion coefficients entering the Toner-Tu like equation Eq. C15:

$$\underline{\beta} = 2.7 \times 10^5 \begin{bmatrix} 1 & 0.58 \\ 1 & 0.58 \end{bmatrix} \mu\text{m}^3/\text{s}. \quad (\text{D6})$$

## Appendix E: Description of the Supplementary Movie

**Supplementary Movie:** Transient evolution of a homogeneous binary mixture into a binary flock upon activation of the colloidal rollers. The system reaches a steady state within ten seconds featuring demixing of the two populations. The confinement diameter is 1.2 mm. The electric field is  $3.4 \text{ V}/\mu\text{m}$ . The  $10 \mu\text{m}$ -diameter colloids are fluorescent and appear bright. The  $7 \mu\text{m}$ -diameter ones appear dark. The video is slowed down 2 times.

- 
- [1] J. C. Crocker and D. G. Grier, Methods of digital video microscopy for colloidal studies, *Journal of colloid and interface science* **179**, 298 (1996).
  - [2] C. Van Der Wel, R. K. Bhan, R. W. Verweij, H. C. Frijters, Z. Gong, A. D. Hollingsworth, S. Sacanna, and D. J. Kraft, Preparation of colloidal organosilica spheres through spontaneous emulsification, *Langmuir* **33**, 8174 (2017).
  - [3] G. E. Pradillo, H. Karani, and P. M. Vlahovska, Quincke rotor dynamics in confinement: rolling and hovering, *Soft Matter* **15**, 6564 (2019).
  - [4] Z. Zhang, H. Yuan, Y. Dou, M. O. De La Cruz, and K. J. Bishop, Quincke oscillations of colloids at planar electrodes, *Physical review letters* **126**, 258001 (2021).
  - [5] A. Bricard, J.-B. Caussin, N. Desreumaux, O. Dauchot, and D. Bartolo, Emergence of macroscopic directed motion in populations of motile colloids, *Nature* **503**, 95 (2013).
  - [6] A. Bricard, J.-B. Caussin, D. Das, C. Savoie, V. Chikkadi, K. Shitara, O. Chepizhko, F. Peruani, D. Saintillan, and D. Bartolo, Emergent vortices in populations of colloidal rollers, *Nature communications* **6**, 7470 (2015).
  - [7] A. Morin and D. Bartolo, Flowing active liquids in a pipe: Hysteretic response of polar flocks to external fields, *Physical Review X* **8**, 021037 (2018).
